# Supplementary material for: WASABI: A Metric for Evaluating Morphometric Plausibility of Synthetic Brain MRIs
Source: arXiv:2504.21771 source file (2025-07-14)
Supplement: Supplementary file 1 [file 8-supp_mat.tex]

\newpage
\appendix

\section{Data}
\label{appendix:data}

\section{Implementations details}
\label{appendix:implementations}
\subsection{Proposed approach implementation details}

\subsection{Comparison methods implementation details}

\section{Supplementary results}
\label{appendix:supp_results}

\section{Supplementary ablations}
\label{appendix:supp_ablations}
